# Supplementary material for: Unsupervised Parameter Efficient Source-free Post-pretraining
Source: arXiv:2502.21313 source file (2025-02-28)
Supplement: Supplementary file 1 [file X_suppl.tex]

\appendix

\section{Overview}
\label{sec:supp_overview}

This supplementary material provides additional analyses and results to complement the main paper. We begin by analyzing the effect of varying the target center vector magnitude (\(\mathbf{s}_{\phi}\)) on model performance, highlighting dataset-specific trends and their impact on feature diversity and discriminability (\cref{sec:supp_target_center_vector}). Next, we extend the analysis of prototype count to additional datasets, exploring its dataset-specific impact and presenting overall performance trends (\cref{sec:supp_nb_prototype}). We then investigate how varying LoRA ranks influence model performance across datasets, emphasizing the importance of dataset-specific rank tuning (\cref{sec:supp_lora_ranks}). Finally, we examine the impact of adapting different combinations of layers (QKV, QKV+Projection, QKV+Projection+MLP) on model performance, identifying the optimal configurations for different datasets (\cref{sec:supp_choice_of_layers}). Each section is supported by visualizations summarizing results across datasets, with a focus on average performance trends to provide a holistic view of our findings.

\section{Selection of Target Center Vector Magnitude}
\label{sec:supp_target_center_vector}

We define $\mathbf{s}_{\phi}$ as the target center vector magnitude, toward which the center vector magnitude is regressed during training, as previously discussed in \cref{sec:loss_reg}. In our experiments, we use a target center vector magnitude of 0.5. In this section, we analyze the effect of different target center vector magnitudes on the model’s performance. We evaluate this on the Flowers102 \cite{nilsback2008automated}, UCF101 \cite{soomro2012ucf101}, and CIFAR100 \cite{krizhevsky2009learning} datasets.

We observe that for both UCF101 and CIFAR10 dataset the target center vector $\mathbf{s}_{\phi}$ of 0.5 leads to the best performance.
As we decrease the value of $\mathbf{s}_{\phi}$, we allow the $L_2$ normalized features to be more spread over the unit-hypersphere, leading to a more diverse feature representation. However, spreading the features all across the unit-sphere can potentially lead to forgetting of the generalized source domain knowledge.
Similarly, an increase in the value of $\mathbf{s}_{\phi}$ leads to a more concentrated feature representation, potentially decreasing the discriminability of the features, and hence the performance of the model is reduced. A $\mathbf{s}_{\phi} = 1$ implies forcing the features to collapse, which is undesirable and hence, we observe the worst performance for this case.
For Flowers102, the model achieves better performance with a target center vector magnitude of 0.2. This suggests that the dataset's distribution is inherently diverse and benefits from a larger feature space to capture its complexity.

\begin{figure}[h]
\centering
\includegraphics[width=\linewidth]{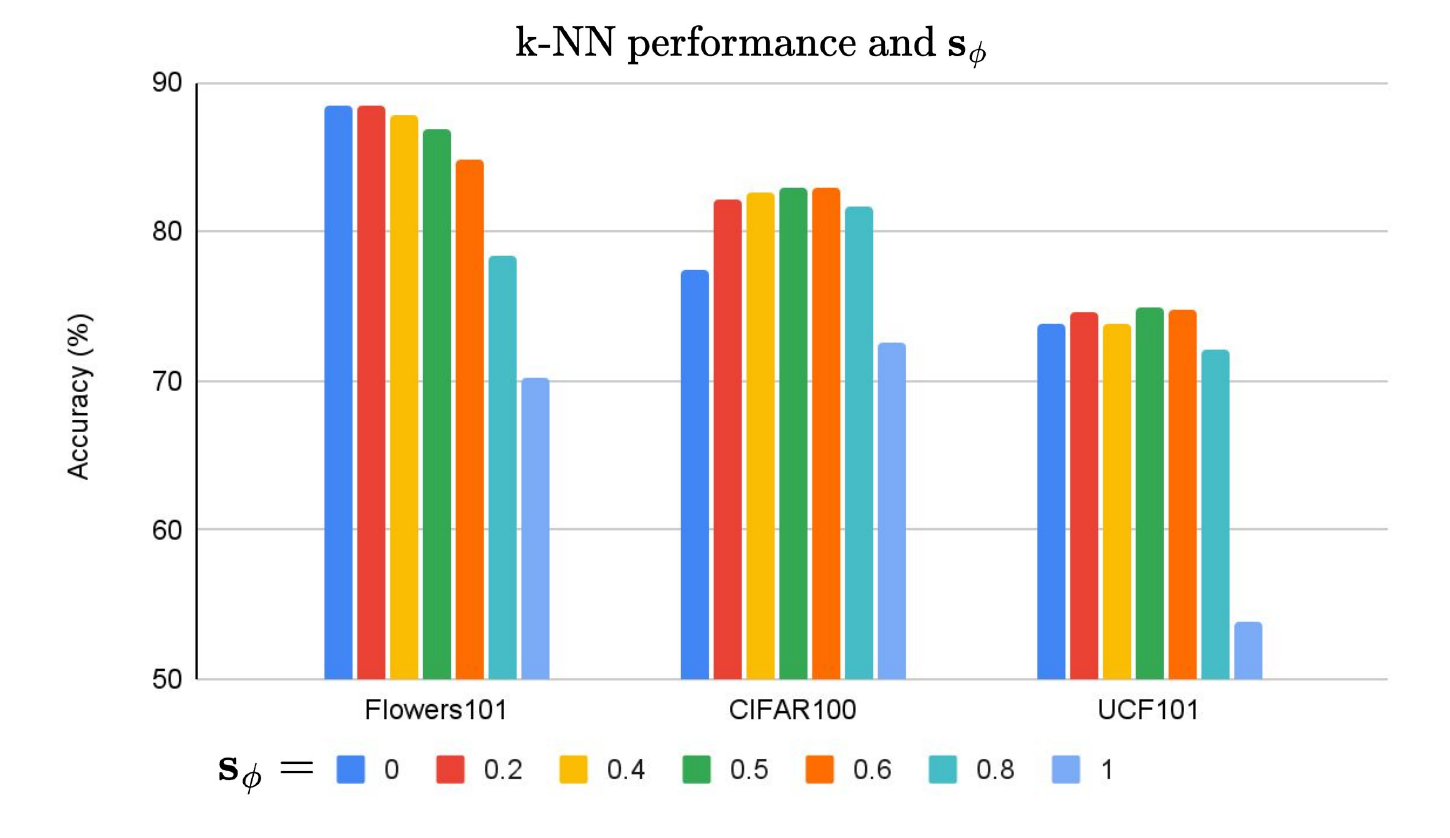}
\caption{
\textbf{Effect of Target Center Vector Magnitude ($\mathbf{s}_{\phi}$) on Model Performance.} 
We evaluate the impact of varying the target center vector magnitude (\(\mathbf{s}_{\phi}\)) on the performance of the model across Flowers102, CIFAR100, and UCF101 datasets.
}
\label{fig:supp_target_center_vector}
\end{figure}

\section{Effect of Number of Prototypes}
\label{sec:supp_nb_prototype}

In \cref{sec:number_of_prototypes}, we analyzed the effect of the number of prototypes on the performance of the un-ensembled model using the Flowers102 dataset. Here, we extend this analysis to additional datasets: CIFAR10, CIFAR100, DTD \cite{cimpoi14describing}, EuroSAT \cite{helber2018introducing}, Oxford-IIIT Pets \cite{parkhi2012cats}, and UCF101. Our findings indicate that the optimal prototype size varies significantly depending on the dataset characteristics.

For smaller and highly distinct target domains like DTD (5k samples across 47 classes), which differs substantially from the source domain (ImageNet \cite{krizhevsky2012imagenet}), increasing the number of prototypes leads to overfitting. Similarly, EuroSAT—a satellite image dataset—shares the characteristic of being very different from the source domain. However, because it has a larger dataset size (27k samples across 10 classes) and fewer classes, overfitting occurs only at higher prototype counts.

Overall, we observe that the optimal number of prototypes is dataset-specific and depends on the target domain's size, diversity, and similarity to the source domain. To provide a holistic view, we present the average performance across all datasets in the bottom-right plot of \cref{fig:supp_nb_prototype}. We observe that overall for all datasets the optimal performance corresponds to the prototype size that is in the middle, i.e. not too small, that can not capture the diversity, and not too large, that can overfit the target training distribution.

\begin{figure*}[h]
\centering
\includegraphics[width=0.9\linewidth]{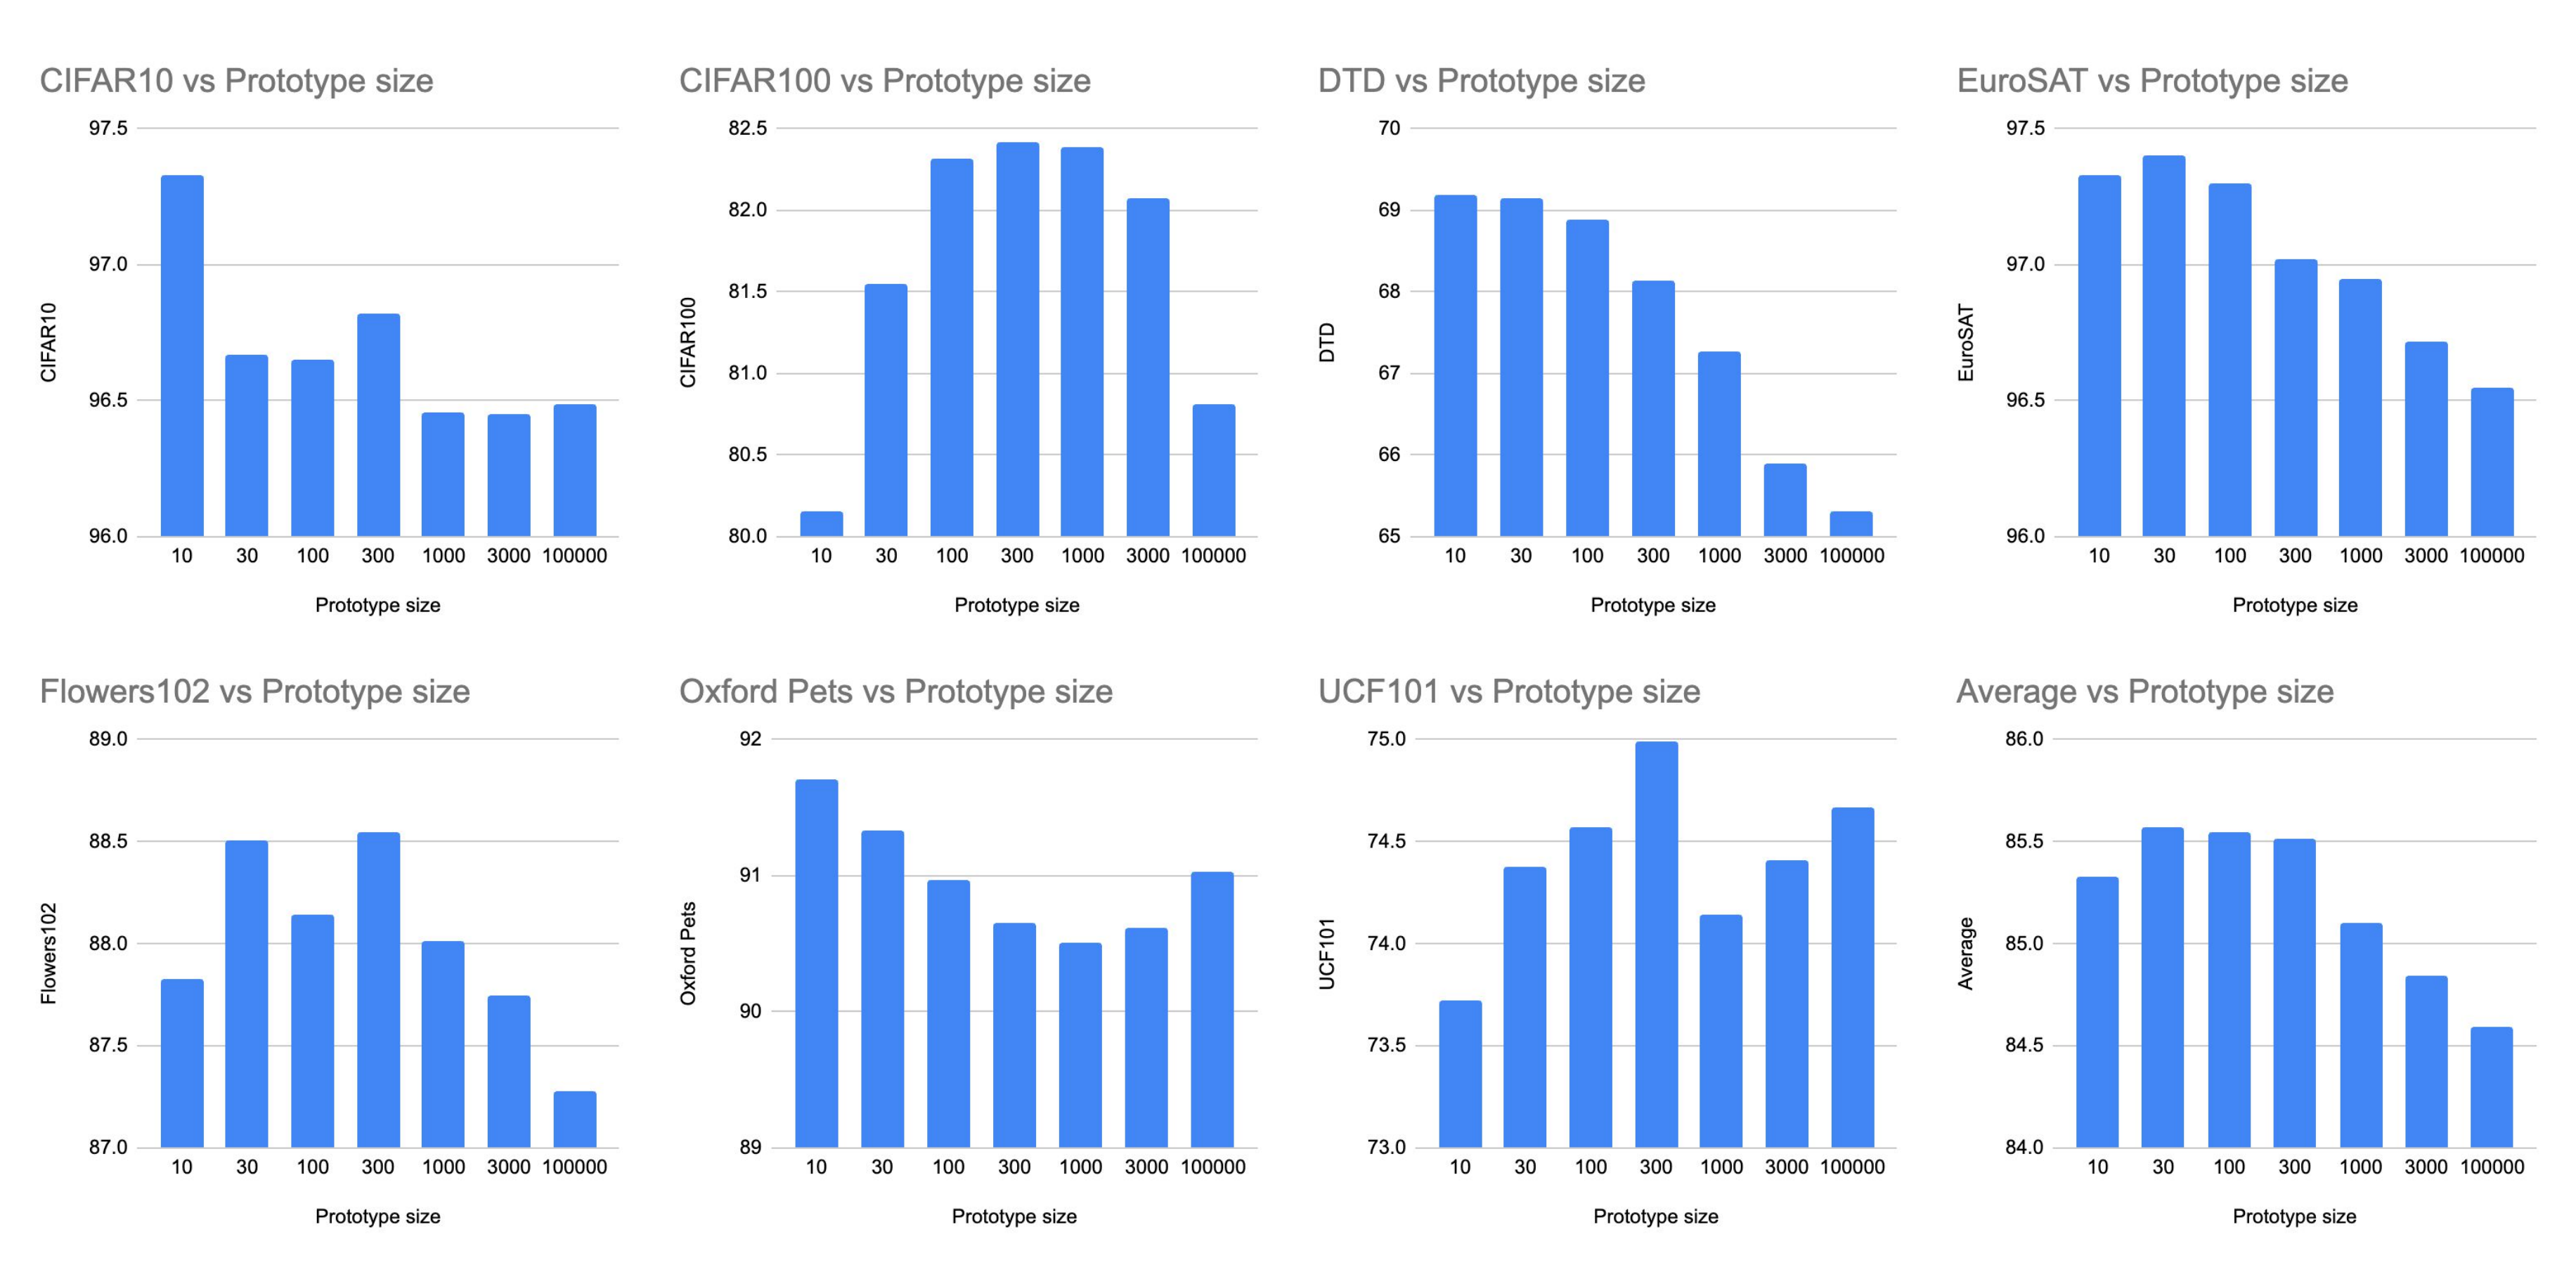}
\caption{
\textbf{Effect of Number of Prototypes on Model Performance.} 
The plot shows the performance of the un-ensembled model across varying numbers of prototypes for CIFAR10, CIFAR100, DTD, EuroSAT, Flowers102, Oxford-IIIT Pets, and UCF101 datasets. The bottom-right sub-plot illustrates the average performance across all datasets.
}
\label{fig:supp_nb_prototype}
\end{figure*}

\section{Effect of Different LoRA Ranks}
\label{sec:supp_lora_ranks}

In this section, we analyze the impact of different LoRA ranks on the performance of the model. Our results indicate that the optimal LoRA rank is dataset-specific, with certain datasets benefiting from lower ranks, while others require higher ranks for optimal performance. The variation highlights the importance of tailoring LoRA ranks to the target domain. To provide a comprehensive view, we present the average performance across all datasets in the bottom-right sub-plot of \cref{fig:supp_lora_ranks}.

\begin{figure*}[h]
\centering
\includegraphics[width=0.9\linewidth]{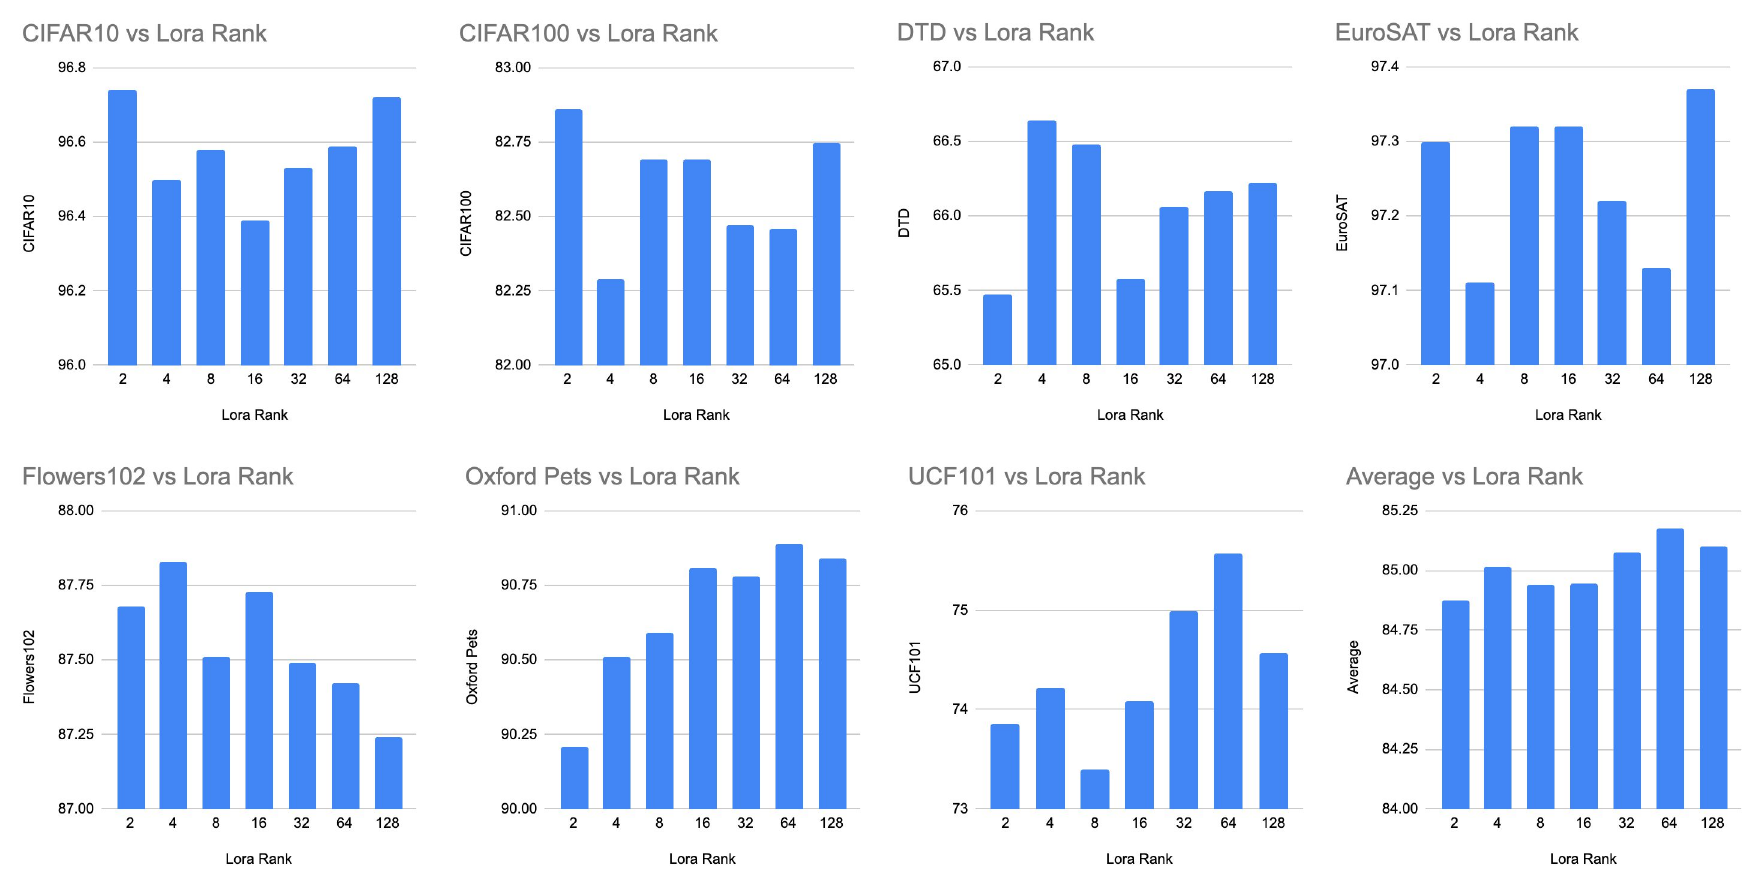}
\caption{
\textbf{Effect of LoRA Ranks on Model Performance.} 
The plot illustrates the performance of the model for varying LoRA ranks across datasets: CIFAR10, CIFAR100, DTD, EuroSAT, Flowers102, Oxford-IIIT Pets, and UCF101. The bottom-right sub-plot shows the average performance across all datasets.
}
\label{fig:supp_lora_ranks}
\end{figure*}

\section{Choice of Layers to Adapt}
\label{sec:supp_choice_of_layers}

In this section, we analyze the effect of the choice of layers to adapt on the performance of the model. Our results show that adapting only the QKV matrices or QKV followed by projection matrices achieves the best performance across all datasets. Adapting QKV, projection, and MLP layers results in slightly lower performance, likely due to the over-parameterization of LoRA parameters. The average performance across all datasets is presented in the bottom-right sub-plot of \cref{fig:supp_choice_of_layers}.

\begin{figure*}[h]
\centering
\includegraphics[width=0.95\linewidth]{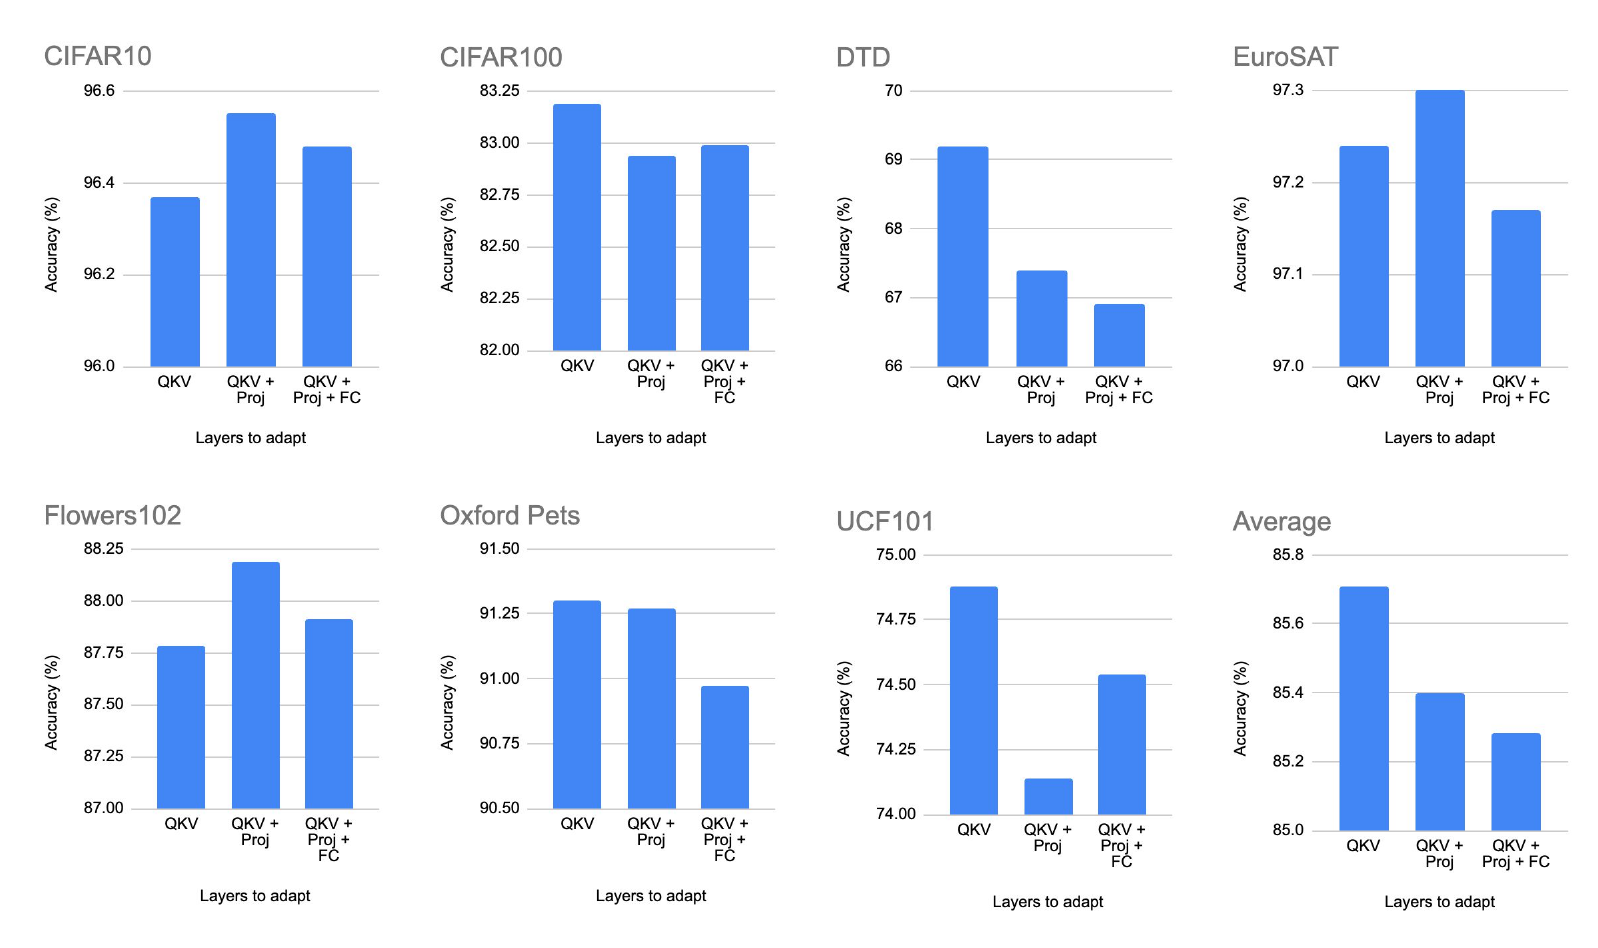}
\caption{
\textbf{Effect of Choice of Layers to Adapt on Model Performance.} 
The plot illustrates the model's performance when adapting different combinations of layers (QKV, QKV+Projection, QKV+Projection+MLP) across datasets: CIFAR10, CIFAR100, DTD, EuroSAT, Flowers102, Oxford-IIIT Pets, and UCF101. The bottom-right sub-plot shows the average performance across all datasets, highlighting that adapting only QKV or QKV+Projection layers achieves the best results.
}
\label{fig:supp_choice_of_layers}
\end{figure*}
